# Supplementary material for: Observation of higher-order exceptional points in pseudo-Hermitian radio-frequency circuits
Source: arXiv:2305.00900 source file (2023-04-18)
Supplement: Supplementary file 1 [file supplementary.pdf]

# Supplemental materials: Observation of higher-order exceptional points in pseudo-Hermitian radio-frequency circuits


Ke Yin, Xianglin Hao, Yuangen Huang, Jianlong Zou, Xikui Ma, and Tianyu Dong*

*School of Electrical Engineering, Xi'an Jiaotong University, Xi'an 710049, China.*


(Dated: April 18, 2023)


In the supplementary materials, the generalized theoretical framework and a comparison of the system's response to perturbations in various scenarios are discussed. In addition, the derivations of the reflection coefficients for conventional and pseudo-Hermitian-trimer-based wireless sensing systems are summarized.


*Generalized Theory* Here, we present a general theoretical analysis for an $n$-dimensional linearly coupled resonator chain, showing that the proposed pseudo-Hermitian system can be extended to higher-dimensional resonator systems where higher-order EP (HOEP) is envisioned. The system illustration is shown in Fig. S1.

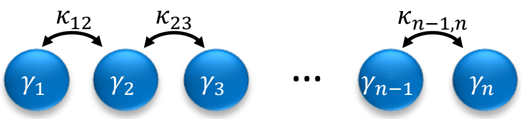


FIG. S1. Illustration of an $n$-dimensional linearly coupled resonator chain where the $m$-th resonator exhibits gain-loss parameter $\gamma_m$ and the coupling coefficient between the $m$-th and $n$-th resonator is $\kappa_{m,n}$.

When only the coupling between adjacent resonators is considered, the chain system can be characterized by a Hamiltonian, which reads

$$\hat{H}_0 = \frac{\omega_0}{2}\begin{pmatrix} 2-\mathrm{i}\gamma_1 & \kappa_{12} & 0 & \cdots & 0 & 0 \\ \kappa_{12} & 2-\mathrm{i}\gamma_2 & \kappa_{23} & \cdots & 0 & 0 \\ 0 & \kappa_{23} & 2-\mathrm{i}\gamma_3 & \cdots & 0 & 0 \\ \vdots & \vdots & \vdots & \ddots & \vdots & \vdots \\ 0 & 0 & 0 & \cdots & \kappa_{n-1,n} & 2-\mathrm{i}\gamma_n \end{pmatrix}, \tag{S1}$$

where $\omega_0$ is the natural resonant frequency of each resonator. With a substitution $\omega = \lambda + \omega_0$, the characteristic equation $\det(\hat{H}_0 - \omega\mathbb{I}_n)$ can be derived, with $\mathbb{I}_n$ being an $n \times n$ identity matrix. For concision, $\omega_0$ is normalized to one hereafter, *i.e.*, $\lambda = \omega/\omega_0 - 1$. The real part of the characteristic equation yields an $n$th-order polynomial in the form of $\lambda^n + b_1\lambda^{n-2} + \ldots + b_{\frac{m_e}{2}}\lambda^{n-m_e} + \ldots$, the coefficients of which are

$$b_{\frac{m_e}{2}} = (-1)^{\frac{m_e}{2}}\frac{1}{2^{m_e}}\left[\sum_{q_1<\ldots<q_{m_e}}\left(\prod_{i=1}^{m_e}\gamma_{q_i}\right) + \ldots + \sum_{\substack{q_{i+1}-q_i=1\\ q_{i+1}<q_{i+2}\\ q_{l+2}<\ldots<q_{m_e}\in\complement_U S}}\left(\prod_{\substack{i=1\\ i\text{ is odd}}}^{l}\kappa^2_{q_iq_{i+1}}\prod_{j=l+2}^{m_e}\gamma_{q_j}\right) + \ldots + \sum_{\substack{q_{i+1}-q_i=1\\ q_{i+1}<q_{i+2}}}\left(\prod_{\substack{i=1\\ i\text{ is odd}}}^{m_e-1}\kappa^2_{q_iq_{i+1}}\right)\right], \tag{S2}$$

where $m_e = 2,4,6,\ldots,n$ [or $(n-1)$ when $n$ is an odd number] with $n$ being an even number; $l = 1,3,5,\ldots,m_e-1$; the sets read $S = \{q_1,q_2,\ldots,q_{l+1}\}$ and $U = \{1,2,\ldots,n\}$; $q_i \in U$ for $i = 1,2,\ldots,n$; and $\complement_U S$ denotes the complement set of $S$ in the complete set $U$. The imaginary part of the characteristic equation yields an $(n-1)$th-order polynomial in the form of $c_1\lambda^{n-1} + c_2\lambda^{n-3} +$

$\ldots + c_{\frac{m_o+1}{2}}\lambda^{n-m_o} + \ldots$, the coefficients of which are

$$c_{\frac{m_o+1}{2}} = (-1)^{\frac{m_o-1}{2}} \frac{1}{2^{m_o}} \left[ \sum_{q_1<\ldots<q_{m_o}} \left( \prod_{i=1}^{m_o} \gamma_{q_i} \right) + \ldots + \sum_{\substack{q_{i+1}-q_i=1 \\ q_{i+1}<q_{i+2} \\ q_{l+2}<\ldots<q_{m_o} \in \complement_U S}} \left( \prod_{\substack{i=1 \\ i \text{ is odd}}}^{l} \kappa^2_{q_i q_{i+1}} \prod_{j=l+2}^{m_o} \gamma_{q_j} \right) + \ldots + \sum_{\substack{q_{i+1}-q_i=1 \\ q_{i+1}<q_{i+2} \\ q_{l+2}<\ldots<q_{m_o} \in \complement_U S}} \left( \prod_{\substack{i=1 \\ i \text{ is odd}}}^{m_o-2} \kappa^2_{q_i q_{i+1}} \gamma_{q_m} \right) \right], \quad \text{(S3)}$$

where $m_o = 1,3,5,\ldots,n-1$ [or $n$ when $n$ is an odd number] with $n$ being an even number; $l = 1,3,5,\ldots,m_o-2$.

In order to satisfy the pseudo-Hermiticity condition, *i.e.*, $\text{Im}[\det(\hat{H}_0 - \omega\mathbb{I}_n)] = 0$, the coefficients (S3) must equal zero. Moreover, the $n$th-order EP exists only when the coefficients (S2) are equal to zero, so that the characteristic equation becomes $\lambda^n_{\text{EPn}} = 0$. The aforementioned conditions result in $n$ equations containing $\gamma_m$ and $\kappa_{m-1,m}$ where $m = 1,\ldots,n$. It should be noted that the coefficients $c_1 = 0$ yield $\sum_{q_1=1}^{n} \gamma_{q_1} = 0$, indicating that the total gain and loss of the system should be balanced. We presume, for the sake of simplicity, that Resonator I is gain with gain parameter $\gamma_1 = -g$, whereas all other resonators have the same loss $g/(n-1)$. The coupling coefficients $(\kappa_{12},\ldots,\kappa_{n-1,n})$ can be calculated by solving the remaining $(n-1)$ equations. Here, we present the eigenfrequency evolution of the four-dimensional and five-dimensional coupled resonator system as a function of $\kappa_{12}$ while maintaining the pseudo-Hermiticity and HOEP conditions for the rest coupling coefficients. As shown in Fig. S2(a) and Fig. S2(b), as $\kappa_{12}$ increases in a four-dimensional system, a fourth-order EP (EP4) characterized by the coalescence of four eigenfrequencies appears. Similarly, a fifth-order EP (EP5) also appears in the five-dimensional system. In both instances, a second-order EP (EP2) is observed in which two of the eigenfrequencies coalesce. Therefore, in an $n$-dimensional coupled resonator system, it is possible to observe EPs with orders less than or equal to $n$.

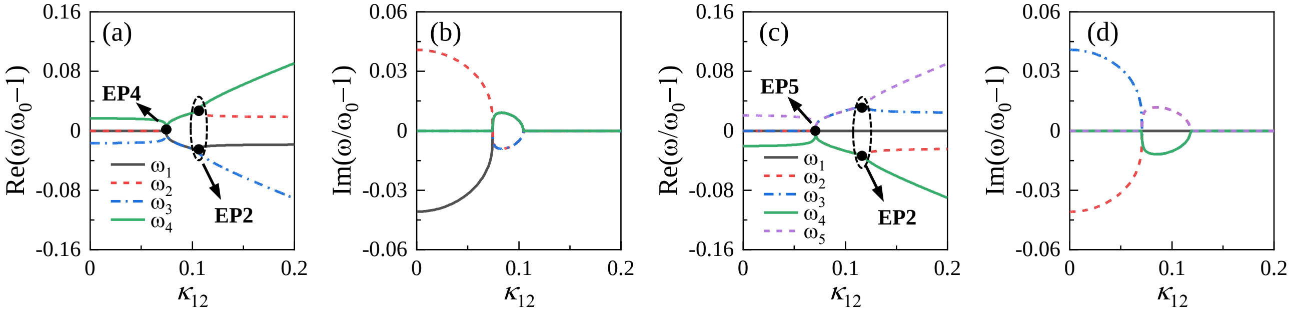


FIG. S2. Eigenfrequency evolution for a (a), (b) four-dimensional and (c), (d) five-dimensional linearly coupled resonator system. The gain parameter is $g = 0.1$.

Figure S3 compares the perturbation behavior of fourth- and fifth-order EPs to the third-order EP. In higher-dimensional systems, the sensitivity is typically dependent on the perturbation's position. To ensure the most significant response, the capacitive perturbation is applied to Resonator II and Resonator III of the four-dimensional and five-dimensional resonator systems, which are biased at EP4 and EP5, respectively. For perturbation at EP4, the perturbed eigenvalues are $\lambda_m = 120^{-1/4} g^{3/4} e^{\text{i}(4m-3)\pi/8} \varepsilon^{1/4} + 30^{-1/2} g^{1/2} e^{-\text{i}(4m-3)\pi/4} \varepsilon^{1/2} + \mathscr{O}(\varepsilon)$, where $m = 1,2,\ldots,n = 4$. As shown in Fig. S3(a) and Fig. S3(b), the eigenfrequencies bifurcate into four branches, with $\lambda_1$ ($\varepsilon > 0$) and $\lambda_2$ ($\varepsilon < 0$) exhibiting the most pronounced response. For perturbation at EP5,the perturbed eigenvalues are $\lambda_m = 7^{-1/5}(g/4)^{4/5} e^{\text{i}(2m-2)\pi/5} \varepsilon^{1/5} - \text{i}(2/5)7^{-4/5}(g/4)^{3/5} e^{-\text{i}(6m-6)\pi/5} \varepsilon^{2/5} + \mathscr{O}(\varepsilon)$, where $m = 1,2,\ldots,n = 5$. Figure S3(c) and Fig. S3(d) demonstrate that the eigenfrequencies bifurcate into five branches, with $\lambda_1$ ($\varepsilon > 0$) and $\lambda_3$ ($\varepsilon < 0$) showing the most significant response. The logarithmic behavior in Fig. S3(f) verifies that the perturbed eigenfrequencies at EP4 and EP5 are dependent on the fourth-root and quintic-root, respectively. The comparison in Fig. S3(e) demonstrates that, despite the fact that the sensitivity of the HOEP-based sensor in response to tiny parameter changes is enhanced as the order of EP increases, it is only effective for a limited range of perturbation parameters. Furthermore, in the EP4-based system, the imaginary part of $\lambda_1$ is larger, resulting in a reduction in the $Q$-factor compared with the EP3- and EP5-based systems.

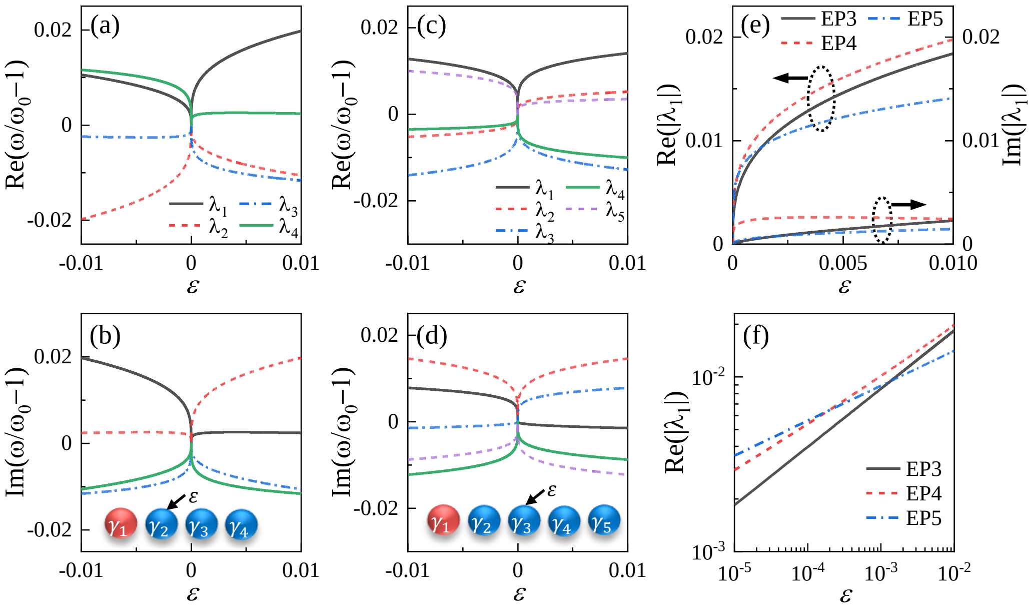


FIG. S3. Perturbation behavior of (a), (b) fourth-order EP and (c), (d) fifth-order EP (e), (f) in comparison with that of third-order EP.

*Perturbation on Resonator III* As discussed in the main text, the complete perturbation Hamiltonian $\hat{H}_p$ of a three-order system can be written as

$$\hat{H}_p = \frac{1}{2}\begin{pmatrix} \varepsilon_1 & 0 & 0 \\ 0 & \varepsilon_2 & 0 \\ 0 & 0 & \varepsilon_3 \end{pmatrix}. \tag{S4}$$

If we consider the case when introducing a capacitive perturbation on Resonator III, *i.e.*, $\varepsilon_1 = \varepsilon_2 = 0$ and $\varepsilon_3 = \varepsilon$, the characteristic equation of the perturbed system $\det(\hat{H}_0 + \hat{H}_p - \omega\mathbb{I}_3) = 0$ at EP3 when $\kappa_{13} = 0$ yields the characteristic equation

$$\lambda^3 - \frac{\varepsilon}{2}\lambda^2 + \mathrm{i}\frac{(\alpha+2)g\varepsilon}{4\left(\alpha^2+3\alpha+2\right)}\lambda - \frac{g^2\varepsilon}{8\left(\alpha^2+3\alpha+2\right)} = 0. \tag{S5}$$

By expanding the eigenvalues with a Newton-Puiseux series $\lambda = c_1\varepsilon^{1/3} + c_2\varepsilon^{2/3}$ and substituting it into the characteristic equation (S5), we have

$$\left(c_2^3 - c_1c_2\right)\varepsilon^2 - \frac{1}{2}c_2^2\varepsilon^{7/3} + \left(3c_2^2c_1 - \frac{c_1^2}{2} + \mathrm{i}\beta c_2 g\right)\varepsilon^{5/3} + \left(3c_2c_1^2 + \mathrm{i}\beta c_1 g\right)\varepsilon^{4/3} + \left[c_1^3 + \frac{g^2\beta}{2(\alpha+2)}\right]\varepsilon = 0, \tag{S6}$$

where $\beta = (\alpha+2)/[4(\alpha^2+3\alpha+2)]$. Solving the last two terms of (S6), *i.e.* $c_1^3 + g^2\beta/[2(\alpha+2)] = 0$ and $3c_2c_1 + \mathrm{i}\beta g = 0$, the coefficients $(c_1, c_2)$ of the Newton-Puiseux series can be obtained. When $\alpha = 1$, the following set of perturbed eigenfrequencies can be derived, which read

$$\lambda_m = \left(\frac{1}{3}\right)^{1/3}\left(\frac{g}{4}\right)^{2/3} e^{\mathrm{i}(2m+1)\pi/3}\varepsilon^{1/3} + \mathrm{i}\frac{1}{2}\left(\frac{1}{3}\right)^{2/3}\left(\frac{g}{4}\right)^{1/3} e^{-\mathrm{i}(2m+1)\pi/3}\varepsilon^{2/3} + \ldots, \tag{S7}$$

where $m = 1, 2, 3$.

Figure S4(a) and S4(b) plot the real and imaginary parts of the perturbed eigenvalues, respectively. When $\varepsilon > 0$, the eigenfrequency with the smallest imaginary part corresponds to the lower frequency branch $\lambda_1$ (black solid line); and it corresponds to the higher frequency branch $\lambda_2$ (red dashed line) when $\varepsilon < 0$. Compared to relay resonator perturbation [see Fig. S4(c)], the frequency bifurcation is diminished, resulting in a reduction in sensitivity. Furthermore, the larger imaginary part [see Fig. S4(d)] indicates a greater resolution loss in the reflection spectrum.

*Perturbation on Resonator I* When a capacitive perturbation on Resonator I is considered, *i.e.*, $\varepsilon_2 = \varepsilon_3 = 0$ and $\varepsilon_1 = \varepsilon$. The characteristic equation of the perturbed system $\det(\hat{H}_0 + \hat{H}_p - \omega\mathbb{I}_3) = 0$ at EP3 when $\kappa_{13} = 0$ yields

$$\lambda^3 - \frac{\varepsilon}{2}\lambda^2 - \mathrm{i}\frac{1}{4}g\varepsilon\lambda + \frac{g^2\varepsilon}{8(\alpha+2)} = 0. \tag{S8}$$

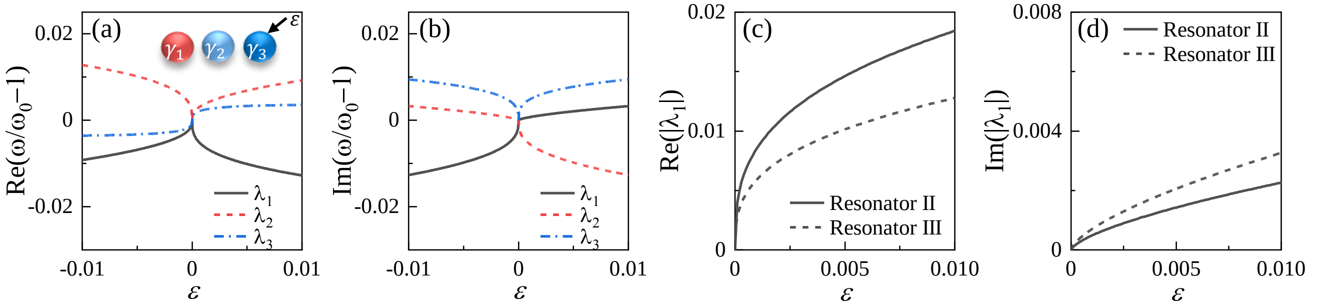


FIG. S4. Theoretical result of the real (a) and imaginary part (b) of the perturbed eigenfrequency evolution of the pseudo-Hermitian system around EP3 when the capacitive perturbation is applied on Resonator III. (c) Comparison of the eigenfrequency bifurcation between Resonator II and III perturbation when $\varepsilon > 0$. Here, $\alpha = 1, g = 0.1$.

By expanding the eigenvalues with a Newton-Puiseux series [1] $\lambda = c_1\varepsilon^{1/3} + c_2\varepsilon^{2/3}$ and substituting it into the characteristic equation (S8), we have

$$\left(c_2^3 - c_1c_2\right)\varepsilon^2 - \frac{1}{2}c_2^2\varepsilon^{7/3} + \left(3c_2^2c_1 - \frac{c_1^2}{2} - \frac{1}{4}\mathrm{i}c_2g\right)\varepsilon^{5/3} + \left(3c_1^2c_2 - \frac{1}{4}\mathrm{i}c_1g\right)\varepsilon^{4/3} + \left[c_1^3 + \frac{g^2}{8(\alpha+2)}\right]\varepsilon = 0. \quad \text{(S9)}$$

Solving the last two terms of (S9), *i.e.*, $c_1^3 + g^2/[8(\alpha+2)] = 0$ and $3c_1c_2 - \mathrm{i}g/4 = 0$, the coefficients $(c_1, c_2)$ of the Newton-Puiseux series can be obtained. When $\alpha = 1$, the following set of perturbed eigenfrequencies are derived, which reads

$$\lambda_m = \left(\frac{2}{3}\right)^{1/3}\left(\frac{g}{4}\right)^{2/3}e^{\mathrm{i}(2m+1)\pi/3}\varepsilon^{1/3} - \mathrm{i}\frac{1}{2}\left(\frac{2}{3}\right)^{2/3}\left(\frac{g}{4}\right)^{1/3}e^{-\mathrm{i}(2m+1)\pi/3}\varepsilon^{2/3} + \ldots, \quad \text{(S10)}$$

where $m = 1, 2, 3$.

As shown in Fig. S5(a) and Fig. S5(b), when perturbing Resonator I, the eigenfrequency with the smallest imaginary part corresponds to $\lambda_1$ when $\varepsilon > 0$ and $\lambda_2$ when $\varepsilon < 0$. Compared to relay resonator perturbation, not only is the frequency bifurcation reduced, but the imaginary part of $\lambda_1$ increases when $\varepsilon > 0$ becomes larger, as shown in Fig. S5(c) and Fig. S5(d), respectively.

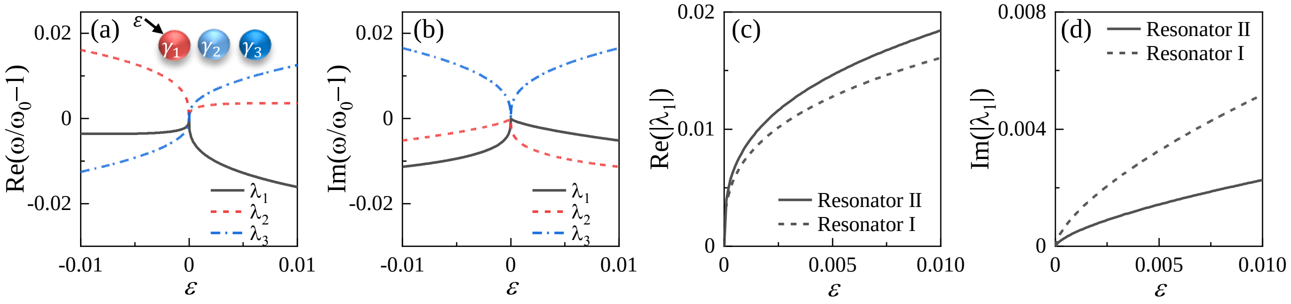


FIG. S5. Theoretical result of the (a) real and (b) imaginary parts of the perturbed eigenfrequency evolution of the pseudo-Hermitian system around EP3 when the capacitive perturbation is applied on Resonator I. (c) Comparison of the Resonator II and I perturbation eigenfrequency bifurcation when $\varepsilon > 0$. Here, $\alpha = 1, g = 0.1$.

*Arbitrary Loss Ratio Between Two Lossy Resonators* Here, we consider a more general situation in which $\alpha \neq 1$, *i.e.*, the loss parameters of the two lossy resonators are distinct. As discussed in the main text, the calculated Newton-Puiseux coefficients for the first perturbed eigenvalue $\lambda_0$ are $c_1 = (1+\alpha)^{-1/3}g^{2/3}/2$ and $c_2 = -\mathrm{i}\alpha(1+\alpha)^{-2/3}g^{1/3}/6$. Figures S6 (a), S6(b) and S6(c), S6(d) illustrate the perturbation behavior of the proposed system when $\alpha = 0.1$ and $\alpha = 10$, respectively. It is evident that $\alpha$ influences the bifurcation of the perturbed eigenvalue. Specifically, due to the fact that both $c_1$ and $c_2$ are decreasing functions of the scaling factor $\alpha$, the bifurcation will decrease as $\alpha$ increases, resulting in a decrease in sensitivity. As shown in Fig. S6(a) and Fig. S6(b), when $\alpha$ is small, such as 0.1, the imaginary part of $\lambda_1$ when $\varepsilon > 0$ and $\lambda_2$ when $\varepsilon < 0$ approaches zero. Thus, as $\alpha$ decreases, the sharpness of the reflection spectrum increases. In the PT-symmetric case where $\alpha = 0$, the system will exhibit a single real mode upon perturbation of a neutral resonator. As shown in Fig. S6(c), the eigenfrequency bifurcation will decrease significantly when $\alpha$ is greater than 1, such as 10. In addition, when $\varepsilon > 0$ ($\varepsilon < 0$), the imaginary part of $\lambda_1$ ($\lambda_2$) becomes larger, indicating poorer spectral resolution. In practical system design, it is necessary to choose the value of the scaling factor $\alpha$ with care.

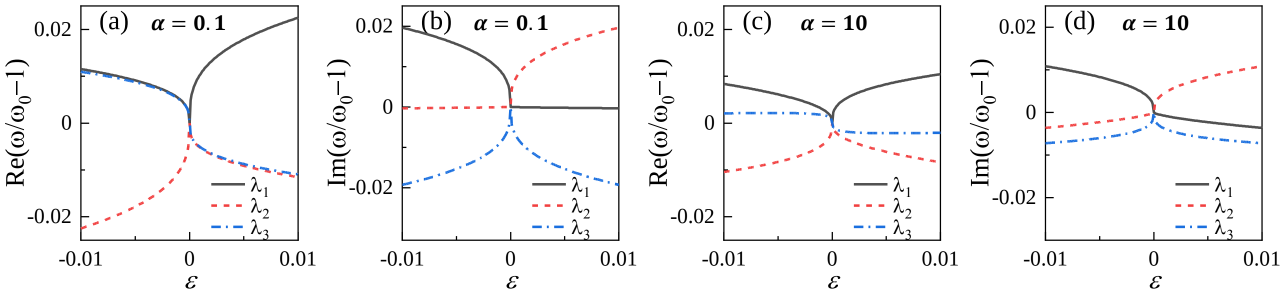


FIG. S6. Perturbation behavior at EP3 when (a), (b) $\alpha = 0.1$ and (c), (d) $\alpha = 10$. The gain parameter is $g = 0.1$.

*Theoretical Reflection Coefficient Derivation* The theoretical reflection coefficient derivation based on circuit theory for both conventional and pseudo-Hermitian-based sensing system is summarized in Table S1. Using the circuit diagram and Kirchhoff's law, the system equations for both cases can be derived. Here, $\omega$ is normalized by the natural resonance frequency $\omega_0 = 1/\sqrt{LC}$; $\gamma = R\sqrt{C/L}$ is the normalized gain/loss parameter; $\kappa = M/L$ is the coupling coefficient; $\varepsilon = -\Delta C/(C+\Delta C)$ is the capacitive perturbation parameter; $\eta = Z_0\sqrt{C/L}$; $\xi = \gamma\omega + \mathrm{i}\left(\omega^2 - 1\right)$; and $Z_0 = 50\ \Omega$ is the intrinsic impedance of the vector network analyzer (VNA).

TABLE S1. Derivation of reflection coefficient of conventional and pseudo-Hermitian wireless sensing system.

| | Conventional | Pseudo-Hermitian trimer |
|---|---|---|
| Schematic | 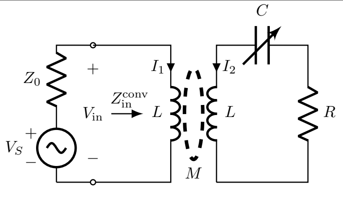  | 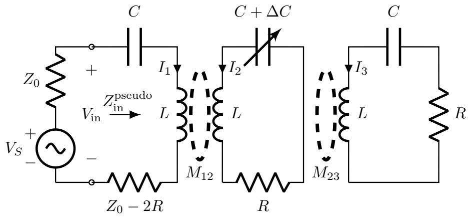  |
| System equation | $\mathrm{i}(\omega - \omega^{-1})I_2 + \gamma I_2 + \mathrm{i}\omega\kappa I_1 = 0$<br>$V_{\mathrm{in}}\gamma/R = \mathrm{i}\omega I_1 + \mathrm{i}\omega\kappa I_2$ | $\mathrm{i}(\omega - \omega^{-1})I_3 + \gamma I_3 + \mathrm{i}\omega\kappa_{23}I_2 = 0$<br>$\mathrm{i}[\omega - \omega^{-1}(1+\varepsilon)]I_2 + \gamma I_2 + \mathrm{i}\omega\kappa_{12}I_1 + \mathrm{i}\omega\kappa_{23}I_3 = 0$<br>$\mathrm{i}(\omega - \omega^{-1})I_1 + (\eta - 2\gamma)I_1 + \mathrm{i}\omega\kappa_{12}I_2 = \gamma V_{\mathrm{in}}/R$ |
| Input impedance | $Z_{\mathrm{in}}^{\mathrm{conv}} = R\dfrac{\omega[\mathrm{i}\gamma\omega - (1-\kappa^2)\omega^2 + 1]}{\gamma[\gamma\omega - \mathrm{i}(1-\omega^2)]}$ | $Z_{\mathrm{in}}^{\mathrm{pseudo}} = Z_0 - 2R + \dfrac{R}{\gamma}\left[\dfrac{\xi\kappa_{12}^2\omega^3}{\kappa_{23}^2\omega^4 + \xi^2 - \mathrm{i}\varepsilon\xi} + \mathrm{i}\left(\omega - \omega^{-1}\right)\right]$ |
| Reflection coefficient | $S_{11} = 20\log_{10}\left\lvert\dfrac{Z_{\mathrm{in}} - Z_0}{Z_{\mathrm{in}} + Z_0}\right\rvert$ | |

---

* Author to whom correspondence should be addressed. Please e-mail to: tydong@mail.xjtu.edu.cn

[1] H. Hodaei, A. U. Hassan, S. Wittek, H. Garcia-Gracia, R. El-Ganainy, D. N. Christodoulides, and M. Khajavikhan, Enhanced sensitivity at higher-order exceptional points, Nature **548**, 187 (2017).
